# Supplementary material for: New Faithfulness-Centric Interpretability Paradigms for Natural Language Processing
Source: arXiv:2411.17992 source file (2024-11-27)
Supplement: Supplementary file 2 [file appendix_leakage.tex]

\section{Explanation of class leakage}
\label{sec:appendix:rroar:leakage}

When importance measures are computed, it is the prediction of the gold label that is explained. For example, for the \emph{Gradient} method, it is $\nabla_\mathbf{x} f(x)_y$ that is computed, where $\mathbf{x}$ is the input and $y$ is the gold label.

We want an importance measure for the correct label, as removing the tokens that are relevant for making a wrong prediction, would help the performance of the model. If the gold label was not used, the faithfulness results would be affected by the model performance. As faithfulness and model performance should be unrelated, this is not a desired outcome.

This is a general issue with faithfulness metrics due to how importance measures are calculated in benchmark settings. This is an unfortunate gap between the benchmark-setting and the practical setting where the gold label is unknown. Furthermore, it is rarely documented.

In ROAR and Recursive ROAR, this issue is expressed as an increase in the model performance. Intuitively, it should not be possible for the model performance to increase with more information removed compared to less. However, because the importance measures are w.r.t. the gold label, they can leak the gold label which can increase the model performance.

\paragraph{Thought experiment.} Consider the SST dataset, a binary sentiment classification task. Let's say that the \texttt{and} token has a spurious correlation with the positive label (there is some truth to this). Although, clearly the \texttt{and} token can appear in both negative and positive sentences.

For example, let's say that just using the \texttt{and} token provides a 60\% accurate classification of positive labels. An importance measure would therefore highlight the \texttt{and} token as being important for the prediction of positive sentiment. Unfortunately, an importance measure might not consider the \texttt{and} token equally important for a negative sentiment (could be due to non-linearity). If all \texttt{and} tokens are removed from sentences with positive sentiment as the gold label, the existence of an \texttt{and} token is now a perfect predictor of negative sentiment. Hence, the model performance will increase (there will still be negative sentiment sentences without \texttt{and} tokens).

Assuming a faithful importance measure, in the next iteration of Recursive ROAR the \texttt{and} token would now be important for predicting negative sentiment and would be removed. However, this assumption is rarely completely justified, there is also no guarantee that \texttt{and} is considered the most important for all observations. Finally, in the case where a relative number of tokens are masked, the removal of other tokens may leak the gold label.

\paragraph{General issue.} As mentioned, the need to use the gold label is a general issue that likely\footnote{We could not find any documentation for which label is used in relevant non-ROAR metrics, and no code has been published.} extends beyond ROAR. However, because ROAR presents a more qualitative metric (\Cref{fig:rroar:roar}) where a curve can be observed to increase, this issue is more apparent. Had we just presented the summarizing metric (\Cref{tab:rroar:faithfulness-metric}), as most faithfulness metrics do, the issue would have been hidden.
