# Supplementary material for: New Faithfulness-Centric Interpretability Paradigms for Natural Language Processing
Source: arXiv:2411.17992 source file (2024-11-27)
Supplement: Supplementary file 7 [file datasets.tex]

\begin{tabular}{lcccccc}
\toprule
Dataset & \multicolumn{3}{c}{Size} & \multicolumn{2}{c}{Inputs} & Performance \\
\cmidrule(r){2-4} \cmidrule(r){5-6}
& Train & Validation & Test & masked & auxilary & class-majority \\
\midrule
bAbI-1 & $8000$ & $2000$ & $1000$ & \texttt{paragraph} & \texttt{question} & $15\%$ \\
bAbI-2 & $8000$ & $2000$ & $1000$ & \texttt{paragraph} & \texttt{question} & $19\%$ \\
bAbI-3 & $8000$ & $2000$ & $1000$ & \texttt{paragraph} & \texttt{question} & $18\%$ \\
BoolQ & $7542$ & $1885$ & $3270$ & \texttt{passage} & \texttt{question} & $62\%$ \\
CB & $200$ & $50$ & $56$ & \texttt{premise} & \texttt{hypothesis} & $22\%$ \\
CoLA & $6841$ & $1710$ & $1043$ & \texttt{sentence} & -- & $0\%$ \\
Anemia & $4262$ & $729$ & $1243$ & \texttt{text} & -- & $39\%$ \\
Diabetes & $8066$ & $1573$ & $1729$ & \texttt{text} & -- & $45\%$ \\
MRPC & $2934$ & $734$ & $408$ & \texttt{sentence1} & \texttt{sentence2} & $41\%$ \\
RTE & $1992$ & $498$ & $277$ & \texttt{sentence1} & \texttt{sentence2} & $47\%$ \\
SST2 & $53879$ & $13470$ & $872$ & \texttt{sentence} & -- & $51\%$ \\
SNLI & $549367$ & $9842$ & $9824$ & \texttt{premise} & \texttt{hypothesis} & $34\%$ \\
IMDB & $20000$ & $5000$ & $25000$ & \texttt{text} & -- & $33\%$ \\
MNLI & $314162$ & $78540$ & $9815$ & \texttt{premise} & \texttt{hypothesis} & $35\%$ \\
QNLI & $83794$ & $20949$ & $5463$ & \texttt{sentence} & \texttt{question} & $51\%$ \\
QQP & $291077$ & $72769$ & $40430$ & \texttt{question1} & \texttt{question2} & $39\%$ \\
\bottomrule
\end{tabular}
