# Supplementary material for: New Faithfulness-Centric Interpretability Paradigms for Natural Language Processing
Source: arXiv:2411.17992 source file (2024-11-27)
Supplement: Supplementary file 11 [file 9-appendix.tex]

\addcontentsline{toc}{compteur}{APPENDICES}

\Annexe{Démo}

\section{AbC}
Texte de l'annexe A\@. Remarquez que la phrase précédente se termine
par une lettre majuscule suivie d'un point. On indique explicitement
cette situation à \LaTeX{} afin que ce dernier ajuste correctement
l'espacement entre le point final de la phrase et le début de la
phrase suivante.
